# Supplementary material for: Quantum key distribution overcoming practical correlated intensity fluctuations
Source: arXiv:2501.13482 source file (2025-01-23)
Supplement: Supplementary file 1 [file SupplementalMaterial.pdf]

# Supplemental Material: Quantum key distribution overcoming practical correlated intensity fluctuations

Jia-Xuan Li,[1,2,*] Ze-Hao Wang,[1,2,*] Feng-Yu Lu,[1,2,*] Víctor Zapatero,[3,4,5] Marcos Curty,[3,4,5] Shuang Wang,[1,2,6,†] Zhen-Qiang Yin,[1,2,6,‡] Wei Chen,[1,2,6] De-Yong He,[1,2,6] Guang-Can Guo,[1,2,6] and Zheng-Fu Han[1,2,6]

[1] *CAS Key Laboratory of Quantum Information, University of Science and Technology of China, Hefei, Anhui 230026, China*
[2] *CAS Center for Excellence in Quantum Information and Quantum Physics, University of Science and Technology of China, Hefei, Anhui 230026, China*
[3] *Vigo Quantum Communication Center, University of Vigo, Vigo E-36310, Spain*
[4] *Escuela de Ingeniería de Telecomunicación, Department of Signal Theory and Communications, University of Vigo, Vigo E-36310, Spain*
[5] *AtlanTTic Research Center, University of Vigo, Vigo E-36310, Spain*
[6] *Hefei National Laboratory, University of Science and Technology of China, Hefei 230088, China*

(Dated: January 23, 2025)

## I. EXPERIMENTAL RESULTS

In this section, we present the experimentally measured data. The experiments for 50 km, 60 km, and 70 km correspond to Tab. I, II, and III, respectively. In the tables, the *Sequence* column refers to the sequence of intensity settings from the current round to the previous three rounds. The first position indicates the current round's setting, while the fourth position shows the setting of the pervious third round. The letters $v$, $d$ and $s$ represent the vacuum state, decoy state and signal state, respectively. The variable $n_X$ denotes the click number in the X basis, $T_X$ represents the error click number in the X basis, and $N_X$ is the send number in the X basis. The same applies to the Z basis. The variable $n_{\text{moni}}$ indicates the click number monitored locally by Alice's local monitor. The following three subsections provide the experimental data for 50 km, 60 km, and 70 km, respectively.

### A. 50km experiment

In the 50km experiment, the average photon number of the signal state is set to 0.24, while the sending probabilities of signal state and decoy state are set to 0.38 and 0.16 respectively. Then, experimentally measured data is shown in Tab. I.

TABLE I: Experimental results for 50km.

| Sequence | $n_X$ | $T_X$ | $N_X$ | $n_Z$ | $T_Z$ | $N_Z$ | $n_{\text{moni}}$ |
|---|---|---|---|---|---|---|---|
| vvvv | 507423 | 55603 | 8497900000 | 487879 | 56109 | 8490800000 | 326416 |
| vvvd | 207471 | 22533 | 3434500000 | 199709 | 22777 | 3431600000 | 134949 |
| vvvs | 417550 | 45160 | 6947400000 | 402663 | 45863 | 6941600000 | 263239 |
| vvdv | 210394 | 23004 | 3532600000 | 202501 | 23427 | 3529600000 | 134575 |
| vvdd | 59391 | 6402 | 1000910000 | 57849 | 6594 | 1000070000 | 36166 |
| vvds | 170638 | 18388 | 2865400000 | 163715 | 18811 | 2862900000 | 109728 |
| vvsv | 431270 | 47260 | 7300800000 | 416225 | 48185 | 7294700000 | 267405 |
| vvsd | 141629 | 15232 | 2374700000 | 136708 | 15543 | 2372700000 | 86851 |
| vvss | 333960 | 36520 | 5613000000 | 320906 | 36586 | 5608300000 | 218049 |
| vdvv | 187777 | 20441 | 3120400000 | 179413 | 20684 | 3117900000 | 112630 |
| vdvd | 72681 | 7895 | 1197170000 | 69763 | 8044 | 1196160000 | 46653 |
| vdvs | 175581 | 19229 | 2904600000 | 168232 | 19206 | 2902100000 | 113691 |
| vddv | 69006 | 7509 | 1157910000 | 67199 | 7698 | 1156950000 | 43263 |
| vddd | 21029 | 2325 | 353260000 | 20305 | 2365 | 352960000 | 13828 |
| vdds | 42271 | 4497 | 706530000 | 40772 | 4580 | 705930000 | 26656 |
| vdsv | 171404 | 18961 | 2865400000 | 164598 | 19012 | 2862900000 | 108992 |
| vdsd | 58997 | 6430 | 981290000 | 56905 | 6497 | 980470000 | 37601 |

* These authors contributed equally to this work
† wshuang@ustc.edu.cn
‡ yinzq@ustc.edu.cn

| | | | | | | | |
|---|---|---|---|---|---|---|---|
| vdss | 111021 | 11902 | 1864440000 | 107204 | 12476 | 1862880000 | 67108 |
| vsvv | 451336 | 49286 | 7457700000 | 433815 | 49495 | 7451500000 | 287000 |
| vsvd | 150038 | 15999 | 2453200000 | 144838 | 16354 | 2451200000 | 97004 |
| vsvs | 369154 | 40214 | 6064300000 | 355242 | 40352 | 6059200000 | 240724 |
| vsdv | 138924 | 15114 | 2315800000 | 134592 | 15403 | 2313900000 | 88629 |
| vsdd | 48544 | 5289 | 804660000 | 46486 | 5335 | 803970000 | 31083 |
| vsds | 117940 | 12794 | 1962570000 | 114357 | 13113 | 1960920000 | 76746 |
| vssv | 380549 | 41219 | 6339100000 | 366710 | 41940 | 6333700000 | 251375 |
| vssd | 133821 | 14430 | 2217700000 | 128736 | 14673 | 2215900000 | 89877 |
| vsss | 304359 | 33099 | 5063500000 | 292689 | 33429 | 5059200000 | 196338 |
| dvvv | 3086531 | 21931 | 2767200000 | 3182943 | 22143 | 2764900000 | 3101100 |
| dvvd | 1555229 | 11069 | 1393420000 | 1605232 | 11192 | 1392250000 | 1561190 |
| dvvs | 2633123 | 18923 | 2374700000 | 2715792 | 19092 | 2372700000 | 2648070 |
| dvdv | 1423169 | 10089 | 1275670000 | 1466647 | 10357 | 1274600000 | 1427490 |
| dvdd | 394770 | 2860 | 353260000 | 406506 | 2796 | 352960000 | 395671 |
| dvds | 781002 | 5612 | 706530000 | 805892 | 5742 | 705930000 | 785970 |
| dvsv | 3159030 | 22630 | 2845700000 | 3258574 | 22974 | 2843300000 | 3180420 |
| dvsd | 1195832 | 8472 | 1079420000 | 1233007 | 8677 | 1078510000 | 1202230 |
| dvss | 2753031 | 19631 | 2492400000 | 2842475 | 20075 | 2490400000 | 2776640 |
| ddvv | 1108637 | 7997 | 1000910000 | 1147118 | 8198 | 1000070000 | 1115580 |
| ddvd | 433271 | 3221 | 392510000 | 444893 | 3093 | 392190000 | 436740 |
| ddvs | 1189564 | 8674 | 1079420000 | 1226960 | 8630 | 1078510000 | 1196830 |
| dddv | 326841 | 2241 | 294390000 | 337477 | 2347 | 294130000 | 329209 |
| dddd | 194669 | 1426 | 176632000 | 200940 | 1411 | 176483000 | 196926 |
| ddds | 238052 | 1672 | 215880000 | 245672 | 1792 | 215710000 | 239954 |
| ddsv | 780200 | 5660 | 706530000 | 804762 | 5792 | 705930000 | 787940 |
| ddsd | 302885 | 2175 | 274760000 | 313044 | 2244 | 274530000 | 305254 |
| ddss | 538866 | 3856 | 490640000 | 554865 | 3945 | 490230000 | 543150 |
| dsvv | 2868038 | 20538 | 2570900000 | 2951581 | 20981 | 2568800000 | 2877890 |
| dsvd | 1066306 | 7686 | 961660000 | 1101360 | 7790 | 960850000 | 1074590 |
| dsvs | 2296997 | 16697 | 2080400000 | 2367096 | 16896 | 2078500000 | 2318710 |
| dsdv | 1115886 | 7946 | 1000910000 | 1149843 | 8013 | 1000070000 | 1123540 |
| dsdd | 217485 | 1595 | 196257000 | 224417 | 1617 | 196092000 | 219810 |
| dsds | 651534 | 4754 | 588780000 | 670463 | 4713 | 588280000 | 656970 |
| dssv | 1950869 | 14009 | 1766320000 | 2008573 | 14053 | 1764830000 | 1964870 |
| dssd | 694797 | 5027 | 628020000 | 715228 | 5168 | 627490000 | 699170 |
| dsss | 1574228 | 11468 | 1432680000 | 1622596 | 11536 | 1431470000 | 1594120 |
| svvv | 36138338 | 89338 | 7614800000 | 36754307 | 84307 | 7608400000 | 36850100 |
| svvd | 12196294 | 30294 | 2570900000 | 12401554 | 28454 | 2568800000 | 12420900 |
| svvs | 28102755 | 69755 | 5966200000 | 28573315 | 66315 | 5961200000 | 28707200 |
| svdv | 11448338 | 28338 | 2414000000 | 11636742 | 26842 | 2411900000 | 11669700 |
| svdd | 4091900 | 10000 | 863530000 | 4164941 | 9541 | 862800000 | 4176540 |
| svds | 10087120 | 24720 | 2139200000 | 10254561 | 23861 | 2137500000 | 10306300 |
| svsv | 27697772 | 67772 | 5828800000 | 28160077 | 65077 | 5823900000 | 28287000 |
| svsd | 7726750 | 19050 | 1628940000 | 7854876 | 18076 | 1627560000 | 7891000 |
| svss | 25954209 | 64209 | 5514800000 | 26400293 | 61293 | 5510100000 | 26602500 |
| sdvv | 11396787 | 28187 | 2414000000 | 11594089 | 26689 | 2411900000 | 11631400 |
| sdvd | 3527725 | 8825 | 745770000 | 3585091 | 8191 | 745150000 | 3592070 |
| sdvs | 11393875 | 28375 | 2433600000 | 11578392 | 26592 | 2431600000 | 11635500 |
| sddv | 4799427 | 11927 | 1020530000 | 4880302 | 11402 | 1019680000 | 4905100 |
| sddd | 745721 | 1761 | 157006000 | 757085 | 1735 | 156873000 | 759620 |
| sdds | 2574936 | 6336 | 549520000 | 2621649 | 6149 | 549050000 | 2629400 |
| sdsv | 9643181 | 23781 | 2041000000 | 9801759 | 22659 | 2039300000 | 9851200 |
| sdsd | 2505113 | 6313 | 529890000 | 2547043 | 5743 | 529450000 | 2559640 |
| sdss | 6878571 | 17471 | 1471930000 | 6991743 | 16343 | 1470690000 | 7047200 |
| ssvv | 28381588 | 71588 | 6123200000 | 28872009 | 68009 | 6118100000 | 29013800 |
| ssvd | 9245155 | 23455 | 2001800000 | 9401125 | 22225 | 2000130000 | 9455600 |
| ssvs | 22189800 | 55800 | 4828000000 | 22577349 | 53349 | 4823900000 | 22730100 |
| ssdv | 10548982 | 26582 | 2276500000 | 10736260 | 25060 | 2274700000 | 10794300 |
| ssdd | 3368398 | 8498 | 726150000 | 3420133 | 8133 | 725550000 | 3442850 |
| ssds | 6861105 | 17305 | 1491560000 | 6982180 | 16280 | 1490290000 | 7030400 |
| sssv | 22515352 | 56352 | 4847600000 | 22894587 | 53587 | 4843500000 | 23062100 |
| sssd | 7622640 | 19240 | 1648550000 | 7747406 | 18206 | 1647170000 | 7806100 |

| | | | | | | | |
|---|---|---|---|---|---|---|---|
| ssss | 17788828 | 45028 | 3866200000 | 18094682 | 42882 | 3863100000 | 18284800 |

## B. 60km experiment

In the 60km experiment, the average photon number of the signal state is set to 0.32, while the sending probabilities of signal state and decoy state are set to 0.20 and 0.19 respectively. Then, experimentally measured data is shown in Tab. II.

TABLE II: Experimental results for 60km.

| Sequence | $n_X$ | $T_X$ | $N_X$ | $n_Z$ | $T_Z$ | $N_Z$ | $n_{\text{moni}}$ |
|---|---|---|---|---|---|---|---|
| vvvv | 926605 | 167725 | 28333000000 | 957823 | 168673 | 28318000000 | 797450 |
| vvvd | 298995 | 54426 | 9103400000 | 298476 | 54075 | 9098600000 | 245173 |
| vvvs | 273345 | 49588 | 8356300000 | 274454 | 49749 | 8351800000 | 224326 |
| vvdv | 300506 | 55231 | 9260700000 | 306398 | 55280 | 9255800000 | 245440 |
| vvdd | 94334 | 16633 | 2811600000 | 93316 | 16745 | 2810100000 | 76750 |
| vvds | 88344 | 15548 | 2615100000 | 87584 | 15709 | 2613700000 | 75621 |
| vvsv | 298738 | 54477 | 9142700000 | 304464 | 54552 | 9137800000 | 248905 |
| vvsd | 82727 | 14542 | 2438000000 | 81201 | 14641 | 2436700000 | 67390 |
| vvss | 90206 | 15996 | 2693600000 | 89262 | 16134 | 2692200000 | 76567 |
| vdvv | 296607 | 54298 | 9064100000 | 303041 | 54051 | 9059200000 | 246042 |
| vdvd | 100329 | 18331 | 3027900000 | 99949 | 18109 | 3026300000 | 76609 |
| vdvs | 81223 | 14749 | 2477400000 | 81272 | 14720 | 2476100000 | 74121 |
| vddv | 94285 | 17324 | 2850900000 | 94663 | 17019 | 2849400000 | 79338 |
| vddd | 37173 | 6315 | 1081400000 | 36410 | 6421 | 1080820000 | 32587 |
| vdds | 28933 | 4985 | 845460000 | 28364 | 4892 | 845010000 | 26410 |
| vdsv | 92568 | 16780 | 2792000000 | 92569 | 16555 | 2790500000 | 77699 |
| vdsd | 27855 | 4733 | 806130000 | 27525 | 4858 | 805700000 | 23888 |
| vdss | 32890 | 5615 | 963430000 | 31823 | 5740 | 962910000 | 26810 |
| vsvv | 287514 | 51704 | 8592200000 | 294953 | 51705 | 8587700000 | 242255 |
| vsvd | 96024 | 16957 | 2831300000 | 95401 | 16826 | 2829800000 | 86737 |
| vsvs | 90549 | 15771 | 2674000000 | 90925 | 16248 | 2672600000 | 79192 |
| vsdv | 86918 | 15508 | 2595300000 | 87549 | 15213 | 2593900000 | 75278 |
| vsdd | 26565 | 4528 | 766810000 | 26286 | 4563 | 766400000 | 21698 |
| vsds | 25249 | 4344 | 727490000 | 24666 | 4292 | 727100000 | 20165 |
| vssv | 93700 | 16775 | 2792000000 | 94268 | 16602 | 2790500000 | 78819 |
| vssd | 34240 | 5749 | 963430000 | 33216 | 5748 | 962910000 | 32158 |
| vsss | 22440 | 3920 | 648840000 | 22141 | 3899 | 648490000 | 20518 |
| dvvv | 7404739 | 98939 | 9123100000 | 7621289 | 87289 | 9118200000 | 11644600 |
| dvvd | 2285791 | 30291 | 2811600000 | 2356474 | 26974 | 2810100000 | 3585220 |
| dvvs | 2540776 | 33776 | 3145900000 | 2617171 | 30371 | 3144200000 | 3989650 |
| dvdv | 1979714 | 26514 | 2438000000 | 2040742 | 23462 | 2436700000 | 3111540 |
| dvdd | 685173 | 9153 | 845460000 | 706674 | 8074 | 845010000 | 1077620 |
| dvds | 873171 | 11731 | 1081400000 | 899792 | 10292 | 1080820000 | 1367900 |
| dvsv | 2050970 | 27080 | 2536400000 | 2110169 | 24469 | 2535100000 | 3235830 |
| dvsd | 791608 | 10618 | 983100000 | 815362 | 9362 | 982570000 | 1246050 |
| dvss | 618538 | 8288 | 766810000 | 636459 | 7359 | 766400000 | 972500 |
| ddvv | 2452919 | 32519 | 3027900000 | 2520772 | 28972 | 3026300000 | 3850090 |
| ddvd | 463116 | 6116 | 570190000 | 475258 | 5478 | 569890000 | 725730 |
| ddvs | 823582 | 11022 | 1022410000 | 847547 | 9777 | 1021870000 | 1301230 |
| dddv | 938523 | 12573 | 1160050000 | 965898 | 11088 | 1159430000 | 1478200 |
| dddd | 285428 | 3918 | 353920000 | 293953 | 3383 | 353730000 | 449620 |
| ddds | 222600 | 2960 | 275260000 | 229253 | 2603 | 275120000 | 349294 |
| ddsv | 761568 | 10178 | 943770000 | 782606 | 9086 | 943260000 | 1195600 |
| ddsd | 270577 | 3647 | 334250000 | 276718 | 3128 | 334070000 | 424700 |
| ddss | 174114 | 2317 | 216280000 | 179984 | 2121 | 216160000 | 274414 |
| dsvv | 2250026 | 30326 | 2772300000 | 2311033 | 26533 | 2770800000 | 3541540 |
| dsvd | 895413 | 12083 | 1101060000 | 920834 | 10724 | 1100480000 | 1410730 |
| dsvs | 509860 | 6800 | 629180000 | 523816 | 5926 | 628840000 | 802530 |
| dsdv | 752964 | 9854 | 924100000 | 774365 | 8965 | 923610000 | 1181350 |
| dsdd | 239160 | 3240 | 294930000 | 247361 | 2771 | 294770000 | 376241 |

| | | | | | | | |
|---|---|---|---|---|---|---|---|
| dsds | 158773 | 2183 | 196618000 | 163546 | 2005 | 196513000 | 251592 |
| dssv | 650244 | 8624 | 806130000 | 668279 | 7849 | 805700000 | 1018120 |
| dssd | 221965 | 2985 | 275260000 | 228013 | 2653 | 275120000 | 350302 |
| dsss | 174207 | 2305 | 216280000 | 178985 | 2078 | 216160000 | 274101 |
| svvv | 33870429 | 237429 | 8336600000 | 34480252 | 190252 | 8332100000 | 53735000 |
| svvd | 11253342 | 78542 | 2772300000 | 11476218 | 63518 | 2770800000 | 17873800 |
| svvs | 11176727 | 78527 | 2772300000 | 11397666 | 63066 | 2770800000 | 17769600 |
| svdv | 11652869 | 82269 | 2870700000 | 11871181 | 65681 | 2869100000 | 18495900 |
| svdd | 4536303 | 32303 | 1120720000 | 4630584 | 25684 | 1120120000 | 7203800 |
| svds | 3482101 | 24701 | 865120000 | 3550968 | 19568 | 864650000 | 5542500 |
| svsv | 9823024 | 69624 | 2418400000 | 10010542 | 55442 | 2417100000 | 15616000 |
| svsd | 2703017 | 19117 | 668510000 | 2754414 | 15114 | 668150000 | 4295800 |
| svss | 3790514 | 27214 | 943770000 | 3871492 | 21492 | 943260000 | 6032100 |
| sdvv | 12086078 | 84578 | 2988600000 | 12292228 | 67428 | 2987000000 | 19174100 |
| sdvd | 3112004 | 21704 | 766810000 | 3166803 | 17303 | 766400000 | 4936600 |
| sdvs | 3184107 | 22407 | 786470000 | 3245252 | 17852 | 786050000 | 5060300 |
| sddv | 2470490 | 17390 | 609510000 | 2511078 | 13878 | 609190000 | 3927850 |
| sddd | 1431029 | 9969 | 353920000 | 1458080 | 7940 | 353730000 | 2272940 |
| sdds | 1505078 | 10708 | 373570000 | 1530862 | 8322 | 373370000 | 2390860 |
| sdsv | 3100309 | 21809 | 766810000 | 3151524 | 17424 | 766400000 | 4933500 |
| sdsd | 1115067 | 7807 | 275260000 | 1134044 | 6274 | 275120000 | 1769930 |
| sdss | 473920 | 3430 | 117971000 | 483396 | 2736 | 117908000 | 754310 |
| ssvv | 10061720 | 70620 | 2516700000 | 10231406 | 56506 | 2515300000 | 15978800 |
| ssvd | 3693387 | 26487 | 924100000 | 3766151 | 20651 | 923610000 | 5865400 |
| ssvs | 2886400 | 20500 | 727490000 | 2943216 | 16316 | 727100000 | 4586700 |
| ssdv | 4092455 | 28655 | 1022410000 | 4161528 | 23128 | 1021870000 | 6491600 |
| ssdd | 1094255 | 7915 | 275260000 | 1118380 | 6290 | 275120000 | 1748750 |
| ssds | 939888 | 6588 | 235940000 | 957515 | 5365 | 235810000 | 1494970 |
| sssv | 2281503 | 16103 | 570190000 | 2320709 | 13009 | 569890000 | 3621180 |
| sssd | 1182245 | 8495 | 294930000 | 1204554 | 6544 | 294770000 | 1877430 |
| ssss | 551276 | 4016 | 137633000 | 561107 | 3207 | 137559000 | 872860 |

### C. 70km experiment

In the 70km experiment, the average photon number of the signal state is set to 0.27, while the sending probabilities of signal state and decoy state are set to 0.15 and 0.15 respectively. Then, experimentally measured data is shown in Tab. III.

TABLE III: Experimental results for 70km.

| Sequence | $n_X$ | $T_X$ | $N_X$ | $n_Z$ | $T_Z$ | $N_Z$ | $n_{\text{moni}}$ |
|---|---|---|---|---|---|---|---|
| vvvv | 1023475 | 264165 | 43941000000 | 997446 | 261246 | 43967000000 | 972150 |
| vvvd | 218620 | 59646 | 9891200000 | 214747 | 58739 | 9897000000 | 186670 |
| vvvs | 214375 | 58510 | 9753900000 | 211126 | 58278 | 9759500000 | 186162 |
| vvdv | 223293 | 59577 | 9930500000 | 218454 | 58700 | 9936300000 | 197984 |
| vvdd | 52477 | 14537 | 2414000000 | 51288 | 14145 | 2415300000 | 41933 |
| vvds | 50147 | 13861 | 2296200000 | 49327 | 13666 | 2297500000 | 42900 |
| vvsv | 233430 | 62404 | 10362200000 | 228505 | 60984 | 10368300000 | 206743 |
| vvsd | 51717 | 14449 | 2394300000 | 50902 | 14013 | 2395700000 | 44116 |
| vvss | 41584 | 11544 | 1923290000 | 41602 | 11467 | 1924420000 | 35371 |
| vdvv | 229557 | 59506 | 9851900000 | 223306 | 58768 | 9857800000 | 216158 |
| vdvd | 45020 | 11962 | 2041100000 | 44641 | 12295 | 2042200000 | 39895 |
| vdvs | 51259 | 14046 | 2335400000 | 51099 | 13882 | 2336800000 | 47866 |
| vddv | 54715 | 14593 | 2433600000 | 53167 | 14366 | 2434900000 | 49614 |
| vddd | 10750 | 2999 | 490640000 | 10661 | 2961 | 490930000 | 9174 |
| vdds | 13253 | 3710 | 608390000 | 13048 | 3624 | 608750000 | 12593 |
| vdsv | 49567 | 13317 | 2198100000 | 48690 | 13162 | 2199300000 | 47215 |
| vdsd | 12747 | 3560 | 588760000 | 12811 | 3524 | 589110000 | 11371 |
| vdss | 12557 | 3502 | 588760000 | 12615 | 3456 | 589110000 | 10751 |
| vsvv | 238473 | 60606 | 10028600000 | 232077 | 59781 | 10034500000 | 236533 |
| vsvd | 51149 | 13638 | 2276600000 | 50453 | 13675 | 2277900000 | 46564 |

| | | | | | | | |
|---|---|---|---|---|---|---|---|
| vsvs | 46910 | 12695 | 2080300000 | 46036 | 12329 | 2081500000 | 43593 |
| vsdv | 51271 | 13536 | 2256900000 | 50079 | 13451 | 2258200000 | 47712 |
| vsdd | 11734 | 3320 | 529880000 | 11437 | 3084 | 530200000 | 10725 |
| vsds | 12184 | 3372 | 569130000 | 12356 | 3391 | 569480000 | 12024 |
| vssv | 50109 | 12956 | 2198100000 | 49645 | 13160 | 2199300000 | 48067 |
| vssd | 11317 | 3062 | 510260000 | 11080 | 3025 | 510560000 | 11043 |
| vsss | 7263 | 2014 | 333630000 | 7188 | 1952 | 333830000 | 6165 |
| dvvv | 4119428 | 70728 | 9989300000 | 4387191 | 71591 | 9995200000 | 10496500 |
| dvvd | 1011264 | 17324 | 2453200000 | 1076947 | 17537 | 2454600000 | 2579830 |
| dvvs | 1014333 | 17363 | 2453200000 | 1080462 | 17482 | 2454600000 | 2578550 |
| dvdv | 923847 | 15757 | 2237300000 | 982097 | 16167 | 2238600000 | 2351820 |
| dvdd | 186282 | 3168 | 451390000 | 197935 | 3092 | 451650000 | 475640 |
| dvds | 186270 | 3292 | 451390000 | 199347 | 3298 | 451650000 | 474630 |
| dvsv | 864576 | 14676 | 2080300000 | 918263 | 14793 | 2081500000 | 2203290 |
| dvsd | 228520 | 3950 | 549510000 | 242867 | 3967 | 549830000 | 579580 |
| dvss | 220391 | 3636 | 529880000 | 234823 | 3733 | 530200000 | 562770 |
| ddvv | 1012563 | 17473 | 2472800000 | 1078541 | 17761 | 2474200000 | 2580250 |
| ddvd | 290669 | 4879 | 706520000 | 310474 | 5034 | 706930000 | 740590 |
| ddvs | 146391 | 2510 | 353260000 | 155851 | 2537 | 353460000 | 371406 |
| dddv | 241820 | 4100 | 588760000 | 258176 | 4196 | 589110000 | 618260 |
| dddd | 64514 | 1145 | 157003000 | 68227 | 1078 | 157095000 | 163196 |
| ddds | 24093 | 413 | 58876000 | 25847 | 413 | 58911000 | 61853 |
| ddsv | 242913 | 4203 | 588760000 | 258649 | 4259 | 589110000 | 619060 |
| ddsd | 64893 | 1121 | 157003000 | 69156 | 1132 | 157095000 | 165154 |
| ddss | 40542 | 709 | 98127000 | 43376 | 706 | 98185000 | 104226 |
| dsvv | 988896 | 17066 | 2414000000 | 1053904 | 17224 | 2415300000 | 2516080 |
| dsvd | 201676 | 3486 | 490640000 | 213980 | 3700 | 490930000 | 513140 |
| dsvs | 161493 | 2829 | 392510000 | 171550 | 2736 | 392740000 | 412379 |
| dsdv | 249309 | 4249 | 608390000 | 266340 | 4400 | 608750000 | 637120 |
| dsdd | 72285 | 1167 | 176629000 | 76993 | 1270 | 176732000 | 185887 |
| dsds | 56355 | 1023 | 137378000 | 59797 | 928 | 137458000 | 143311 |
| dssv | 210258 | 3621 | 510260000 | 222659 | 3669 | 510560000 | 533570 |
| dssd | 81394 | 1416 | 196254000 | 86257 | 1369 | 196369000 | 205907 |
| dsss | 32671 | 577 | 78502000 | 34957 | 539 | 78548000 | 83339 |
| svvv | 20777888 | 116888 | 9655700000 | 20322002 | 117002 | 9661300000 | 52411000 |
| svvd | 4950407 | 27907 | 2296200000 | 4836909 | 28009 | 2297500000 | 12486800 |
| svvs | 5316377 | 29777 | 2472800000 | 5191413 | 30213 | 2474200000 | 13387300 |
| svdv | 4438727 | 24827 | 2060700000 | 4339591 | 24891 | 2061900000 | 11190700 |
| svdd | 1437388 | 8088 | 667260000 | 1404925 | 8015 | 667650000 | 3628530 |
| svds | 1346514 | 7594 | 628010000 | 1316500 | 7700 | 628380000 | 3397920 |
| svsv | 4199874 | 23574 | 1942910000 | 4107697 | 23497 | 1944060000 | 10596900 |
| svsd | 891046 | 5016 | 412140000 | 869682 | 4962 | 412380000 | 2247160 |
| svss | 1267368 | 7118 | 588760000 | 1235461 | 7231 | 589110000 | 3190480 |
| sdvv | 5482744 | 30644 | 2570900000 | 5371626 | 31226 | 2572400000 | 13856800 |
| sdvd | 845181 | 4891 | 392510000 | 824584 | 4924 | 392740000 | 2127740 |
| sdvs | 1007249 | 5709 | 471010000 | 984280 | 5700 | 471290000 | 2539810 |
| sddv | 1093272 | 6232 | 510260000 | 1067207 | 6057 | 510560000 | 2755360 |
| sddd | 336123 | 1903 | 157003000 | 328673 | 1993 | 157095000 | 848970 |
| sdds | 379553 | 2203 | 176629000 | 369222 | 2142 | 176732000 | 954670 |
| sdsv | 1093990 | 6130 | 510260000 | 1071408 | 6238 | 510560000 | 2761340 |
| sdsd | 379283 | 2123 | 176629000 | 371740 | 2190 | 176732000 | 958690 |
| sdss | 210703 | 1223 | 98127000 | 205787 | 1117 | 98185000 | 532650 |
| ssvv | 4166970 | 23470 | 1982170000 | 4076294 | 23894 | 1983330000 | 10507100 |
| ssvd | 1242693 | 7083 | 588760000 | 1214452 | 6952 | 589110000 | 3124140 |
| ssvs | 992305 | 5795 | 471010000 | 970311 | 5731 | 471290000 | 2500430 |
| ssdv | 1197935 | 6925 | 569130000 | 1172783 | 6963 | 569480000 | 3019400 |
| ssdd | 289806 | 1626 | 137378000 | 283241 | 1621 | 137458000 | 732730 |
| ssds | 165945 | 980 | 78502000 | 162153 | 973 | 78548000 | 418320 |
| sssv | 707237 | 4097 | 333630000 | 691741 | 4061 | 333830000 | 1783480 |
| sssd | 167491 | 967 | 78502000 | 164159 | 927 | 78548000 | 422570 |
| ssss | 42191 | 230 | 19625400 | 40732 | 241 | 19636900 | 104699 |
